# Supplementary material for: Competitive Retrieval: Going Beyond the Single Query
Source: arXiv:2404.09253 source file (2024-04-14)
Supplement: Supplementary file 1 [file prompts-features.tex]

\begin{tabular}{|l|l|p{6cm}|c|}
\hline
\textbf{Feature Category} & \textbf{Feature Name} & \textbf{Description} & \textbf{Number of Positive Labels} \\ \hline
Competition Framework & Competition Background & Explanation of score calculation (based on the median rank). & 3 \\ \cline{2-4}
Competition Framework & Competition Instructions & Guidelines for document creation, such as not to add links or use keyword stuffing. & 8 \\ \hline
Query and Topic Focus & Topic Name & Inclusion of the topic name only. & 10 \\ \cline{2-4}
Query and Topic Focus & 3 Queries & Prompt containing all three query variations. & 29 \\ \cline{2-4}
Query and Topic Focus & 1 Query Only & Inclusion of only one out of the three queries. & 3 \\ \hline
Document and Rank Reference & Initial Document & Inclusion of the initial document as a specific starting point or example. & 2 \\ \cline{2-4}
Document and Rank Reference & Own Previous Ranks & Inclusion of the student's previous ranks in the competition. & 7 \\ \cline{2-4}
Document and Rank Reference & Previous Document & Inclusion of the student's previous document. & 9 \\ \cline{2-4}
Document and Rank Reference & Only Previous Winner Document & Inclusion of the previous winners documents only. & 18 \\ \cline{2-4}
Document and Rank Reference & All Documents From Previous Round & Inclusion of all five documents from the previous round along with their rankings. & 5 \\ \cline{2-4}
Document and Rank Reference & All Higher Ranked Documents & Inclusion of documents from the previous round that ranked higher than the student's document. & 2 \\ \hline
Strategy & Instruction To Get Closer To Winner & Specific prompt to create a document similar to (at least one) of the previous winners. & 16 \\ \cline{2-4}
Strategy & Instruction To Keyword Stuffing & Prompt instructing to perform keyword stuffing. & 8 \\ \cline{2-4}
Strategy & Improve Worst Query & Focus on the worst performing query from the last round, either by including only this query or instructing to improve a document to rank higher in this query. & 9 \\ \cline{2-4}
Strategy & Improve Best Query & Similar to 'Improve Worst Query' but focusing on the best performing query from the last round. & 1 \\ \hline
\end{tabular}
