# Supplementary material for: Competitive Retrieval: Going Beyond the Single Query
Source: arXiv:2404.09253 source file (2024-04-14)
Supplement: Supplementary file 2 [file competition-background-_score-calculation_.tex]

\begin{table}
\caption{3 prompts}
\label{tab: competition-background-(score-calculation)}
\begin{tabular}{lrrrr}
\toprule
 & avg rank & median rank & raw promotion & scaled promotion \\
\midrule
with strategy & \bfseries 1.864 & \bfseries 1.963 & \bfseries 0.037 & \bfseries 0.056 \\
without strategy & \color{blue} \underline{2.841} & \color{blue} \underline{2.910} & \color{blue} -0.077 & \color{blue} -0.023 \\
students & \color{blue} \underline{2.675} & \color{blue} \underline{2.674} & \color{blue} 0.012 & \color{blue} 0.003 \\
dummy & \color{blue} \underline{3.419} & \color{blue} \underline{3.415} & \color{blue} -0.058 & \color{blue} \underline{-0.067} \\
\bottomrule
\end{tabular}
\end{table}
